# Supplementary material for: A general framework for nonlocal traffic flow models on networks
Source: arXiv:2607.09227 source file (2026-07-10)
Supplement: Supplementary file 3 [file dat_20260612-001355-545_s2_c2_SI.tex]

\def\rs{5,6}
\def\intervals{1.525/6.6}

% Generated by user 'florian' from network with OID '20260612-001355-545' with MATLAB version '25.1.0.2973910 R2025a Update 1' on date_time '2026-06-12_21-57-50'.
