# Supplementary material for: A general framework for nonlocal traffic flow models on networks
Source: arXiv:2607.09227 source file (2026-07-10)
Supplement: Supplementary file 5 [file dat_20260612-001510-494_s1_c1_SI.tex]

\def\rs{2,3}
\def\intervals{1/7.2}

% Generated by user 'florian' from network with OID '20260612-001510-494' with MATLAB version '25.1.0.2973910 R2025a Update 1' on date_time '2026-06-12_12-06-50'.
